# Supplementary material for: After the Fix: Transfer of Corrected Agent Experience
Source: arXiv:2609.34603 source file (2026-09-29)
Supplement: Supplementary file 1 [file consistency.tex]

ThinkingBox & 61 & 42 & 18 & 15 & 1 & 0 \\
APEX-state & 29 & 5 & 1 & 22 & 6 & 1 \\
APEX-text & 22 & 6 & 1 & 28 & 7 & 1 \\
