# Supplementary material for: After the Fix: Transfer of Corrected Agent Experience
Source: arXiv:2609.34603 source file (2026-09-29)
Supplement: Supplementary file 2 [file contrasts.tex]

TB & C-F / U-F & 46/2 & +44 & [25.3, 56.3] & $<0.0001$ & $<0.0001$ & $<0.0001$ \\
TB & C-S / U-S & 39/10 & +29 & [12.7, 39.8] & $<0.0001$ & 0.0003 & 0.0008 \\
TB & C-H / U-H & 36/4 & +32 & [19.1, 44.0] & $<0.0001$ & $<0.0001$ & $<0.0001$ \\
TB & C-F / B & 31/6 & +25 & [13.1, 37.7] & $<0.0001$ & 0.0004 & 0.0009 \\
TB & C-S / B & 30/8 & +22 & [8.0, 39.0] & 0.0005 & 0.0038 & 0.0094 \\
TB & C-H / B & 24/6 & +18 & [6.7, 32.5] & 0.0014 & 0.0100 & 0.0272 \\
TB & E / S & 15/4 & +11 & [1.4, 18.9] & 0.0192 & 0.0961 & 0.3266 \\
TB & C-F / E & 7/7 & +0 & [-6.4, 6.1] & 1.0000 & 1.0000 & 1.0000 \\
State & C-F / U-F & 8/9 & -1 & [-7.8, 5.4] & 1.0000 & 1.0000 & 1.0000 \\
State & C-S / U-S & 15/12 & +3 & [-5.1, 10.6] & 0.7011 & 1.0000 & 1.0000 \\
State & C-H / U-H & 12/8 & +4 & [-6.0, 13.5] & 0.5034 & 1.0000 & 1.0000 \\
State & C-F / B & 10/13 & -3 & [-13.3, 5.6] & 0.6776 & 1.0000 & 1.0000 \\
State & C-S / B & 12/14 & -2 & [-10.5, 7.1] & 0.8450 & 1.0000 & 1.0000 \\
State & C-H / B & 11/10 & +1 & [-7.1, 9.7] & 1.0000 & 1.0000 & 1.0000 \\
State & E / S & 12/8 & +4 & [-5.3, 13.3] & 0.5034 & 1.0000 & 1.0000 \\
State & C-F / E & 11/14 & -3 & [-13.3, 6.5] & 0.6900 & 1.0000 & 1.0000 \\
Text & C-F / U-F & 10/10 & +0 & [-7.4, 6.2] & 1.0000 & 1.0000 & 1.0000 \\
Text & C-S / U-S & 14/13 & +1 & [-9.9, 13.0] & 1.0000 & 1.0000 & 1.0000 \\
Text & C-H / U-H & 5/13 & -8 & [-16.7, 1.9] & 0.0963 & 0.5775 & 1.0000 \\
Text & C-F / B & 11/13 & -2 & [-14.4, 9.4] & 0.8388 & 1.0000 & 1.0000 \\
Text & C-S / B & 9/11 & -2 & [-10.3, 7.2] & 0.8238 & 1.0000 & 1.0000 \\
Text & C-H / B & 7/14 & -7 & [-15.7, 2.1] & 0.1892 & 1.0000 & 1.0000 \\
Text & E / S & 14/2 & +12 & [3.2, 22.5] & 0.0042 & 0.0251 & 0.0753 \\
Text & C-F / E & 5/12 & -7 & [-19.8, 4.1] & 0.1435 & 0.5739 & 1.0000 \\
