# Supplementary material for: After the Fix: Transfer of Corrected Agent Experience
Source: arXiv:2609.34603 source file (2026-09-29)
Supplement: Supplementary file 3 [file influence.tex]

ThinkingBox & C-F / U-F & 15 & +40.66 & +48.42 \\
ThinkingBox & C-S / U-S & 15 & +25.27 & +31.96 \\
ThinkingBox & C-H / U-H & 15 & +27.78 & +34.74 \\
ThinkingBox & E / S & 15 & +8.64 & +13.33 \\
APEX-state & C-F / U-F & 16 & -2.22 & +1.08 \\
APEX-state & C-S / U-S & 16 & +1.05 & +4.30 \\
APEX-state & C-H / U-H & 16 & +1.06 & +6.19 \\
APEX-state & E / S & 16 & +0.00 & +5.43 \\
APEX-text & C-F / U-F & 16 & -1.14 & +2.13 \\
APEX-text & C-S / U-S & 16 & -1.08 & +4.55 \\
APEX-text & C-H / U-H & 16 & -10.53 & -5.68 \\
APEX-text & E / S & 16 & +8.51 & +13.98 \\
