# Supplementary material for: After the Fix: Transfer of Corrected Agent Experience
Source: arXiv:2609.34603 source file (2026-09-29)
Supplement: Supplementary file 4 [file resources.tex]

ThinkingBox & B-only & 42 & 0.232 & 9.48 & 24.4 & 14.96 \\
ThinkingBox & Summary & 56 & 0.264 & 9.48 & 27.9 & 17.09 \\
ThinkingBox & Execution & 67 & 0.353 & 9.27 & 38.1 & 18.34 \\
ThinkingBox & C-Full & 67 & 0.434 & 8.85 & 49.0 & 17.07 \\
ThinkingBox & C-Skill & 64 & 0.286 & 9.80 & 29.2 & 17.61 \\
ThinkingBox & C-Hybrid & 60 & 0.318 & 9.82 & 32.4 & 17.44 \\
APEX-state & B-only & 44 & 2.189 & 37.78 & 58.0 & 46.47 \\
APEX-state & Summary & 40 & 2.307 & 43.01 & 53.6 & 56.51 \\
APEX-state & Execution & 44 & 2.405 & 41.22 & 58.4 & 54.92 \\
APEX-state & C-Full & 41 & 2.737 & 20.04 & 136.6 & 22.83 \\
APEX-state & C-Skill & 42 & 2.337 & 39.19 & 59.6 & 48.50 \\
APEX-state & C-Hybrid & 45 & 2.273 & 37.39 & 60.8 & 46.46 \\
APEX-text & B-only & 47 & 2.227 & 37.51 & 59.4 & 46.19 \\
APEX-text & Summary & 40 & 2.172 & 37.29 & 58.3 & 45.72 \\
APEX-text & Execution & 52 & 2.438 & 35.08 & 69.5 & 44.40 \\
APEX-text & C-Full & 45 & 3.576 & 30.01 & 119.2 & 38.24 \\
APEX-text & C-Skill & 45 & 2.383 & 40.46 & 58.9 & 48.97 \\
APEX-text & C-Hybrid & 40 & 2.236 & 37.22 & 60.1 & 45.75 \\
