# Supplementary material for: After the Fix: Transfer of Corrected Agent Experience
Source: arXiv:2609.34603 source file (2026-09-29)
Supplement: Supplementary file 5 [file triples.tex]

000 & 26 & 22 & 31 & 43 & 40 & 42 & 38 & 37 & 38 \\
001 & 24 & 21 & 16 & 4 & 7 & 6 & 5 & 5 & 2 \\
010 & 1 & 6 & 3 & 3 & 4 & 3 & 4 & 7 & 8 \\
011 & 7 & 9 & 8 & 6 & 5 & 5 & 6 & 4 & 5 \\
100 & 5 & 4 & 5 & 7 & 6 & 5 & 7 & 5 & 9 \\
101 & 22 & 18 & 20 & 4 & 8 & 6 & 5 & 9 & 3 \\
110 & 1 & 4 & 1 & 6 & 8 & 5 & 6 & 6 & 5 \\
111 & 14 & 16 & 16 & 27 & 22 & 28 & 29 & 27 & 30 \\
